# Supplementary material for: ManiFPT: Defining and Analyzing Fingerprints of Generative Models
Source: arXiv:2402.10401 source file (2024-02-29)
Supplement: Supplementary file 1 [file fig-suppl-viz-art-rgb-gm256.tex]

\begin{figure}[thb]
  \centering
  \includegraphics[width=\linewidth]{figs/suppl-viz-art-rgb-triplets-gm256.png}
  \caption{Visualization of artifacts in RGB space under our definition (Sec.\ref{defn:artifact}) from \gmchq{} dataset: generated image ($x_G$), closest point on the data manifold ($x^{\star}$) in RGB space, and artifact ($a$) }
  % \Description{A woman and a girl in white dresses sit in an open car.}
  \label{fig:suppl-viz-art-rgb-triplets-gm256}
\end{figure}
